# Supplementary material for: Data-driven modeling and control of large-scale dynamical systems in the Loewner framework
Source: arXiv:2108.11870 source file (2021-08-26)
Supplement: Supplementary file 1 [file sec-appendix.tex]

The following relations have been considered: $B_0=b+2H_0\tan(\alpha)$, $S_0=H_0(b+H_0\tan(\alpha)$, $V_0=\frac{Q_0}{S_0}$, $\delta_0=c_0^2-V_0^2$, $\beta_0=gS_0\mu_0$, $\gamma_0=g\big(I-J_0-\eta_0 -\frac{S_0\rho_0}{B_0} \big)$, $\varphi_0=\frac{\gamma_0}{2}$, $c_0=\sqrt{\frac{gS_0}{B_0}}$, $\Phi_0=2\varphi_0V_0+\beta_0\delta_0$, $\mu_0=\frac{2}{K_s^2}W_0Q_0$, $W_0=\big( \frac{P_0^2}{S_0^5}\big)^{2/3}$, $P_0=b+aH_0$, $a=2/\cos(\alpha)$, $J_0=W_0\big( \frac{Q_0}{K_s}\big)^2$, $\eta_0=\frac{I-J_0}{1-\frac{B_0Q_0^2}{gS_0^3}}$, $\rho_0=\frac{2}{3}\big(\frac{Q_0}{K_s}\big)^2W_0\big( 2\frac{a}{P_0}-5\frac{B_0}{S_0}\big)$.
